# Supplementary material for: What Makes a Good Commit Message?
Source: arXiv:2202.02974 source file (2022-02-07)
Supplement: Supplementary file 1 [file table_appendixB.tex]

\begin{table*}
\centering
\caption{Details of ``What" expression categories}
\begin{adjustbox}{angle=90}
    \begin{tabular}{p{2.5cm}p{3.5cm}<{\centering}p{8cm}p{1.5cm}<{\centering}p{6cm}}
  
    \toprule
    Category & Subcategory & Explanation & Statistic & Example\\
    \midrule
    
    \multirow{3}*{\shortstack{Summarize \\Code \\Object\\ Change}} & Characteristics of changes & Highlight the characteristics of the current code change and comparing them with other implementation methods to summarize the code changes & 13(5.2\%) & \textit{``attempt at a 3rd I/O interface [...] inspired by InputStream and OutputStream, but using growing buffers instead of byte arrays as the core data container''}\\
    
     & Object of change & Summarize the changes from the point of view of the code objects  & 143(56.8\%) & \textit{``remove creation of `fat' jar...''}\\
    
     & Change list & Indicate changes of several code objects, involving one or more source files & 6(2.4\%) & \textit{``this commit removes the following deprecated properties: * `server.connection-timeout' * `server.use-forward-headers' [...]''} \\
    
     & Contrast before and after & Contrast the state of code objects before and after changes & 16(6.4\%) & \textit{``rename HeldCertificate.Builder.issuedBy() to signedBy()''}\\
    \midrule
    
     \multirow{1}*{\shortstack{Describe \\Implementation \\Principle}} & - & Represent commit messages describing technical principles underpinning the changes & 6(2.4\%)& \textit{``SslContextBuilder was using InetAddress.getByName(null) [...] On Android, null returns IPv6 loopback, which has the name `ip6-localhost' ''} \\
    \midrule
    
     \multirow{1}*{\shortstack{Illustrate \\Function}} & - & Summarize and explain code changes from a functional perspective & 65(25.8\%)& \textit{``Rename preferred-mapper property so its clear it only applies to JSON''} \\
    \midrule
     \multirow{1}*{\shortstack{Missing \\What}} & - & Refer to commit messages that lack any specification of what was changed & 19(7.5\%)& \textit{``fix typo''}\\
    \bottomrule 
    \end{tabular} 
\end{adjustbox}
\label{what (sub)categories information}
\end{table*}
