# Supplementary material for: What Makes a Good Commit Message?
Source: arXiv:2202.02974 source file (2022-02-07)
Supplement: Supplementary file 2 [file appendix.tex]

\begin{table*}
\centering
\caption{Details of ``Why" categories}
\begin{adjustbox}{angle=90}
    \begin{tabular}{p{1.7cm}p{3.5cm}<{\centering}p{8cm}p{1.5cm}<{\centering}p{6cm}}
  
    \toprule
    Category & Subcategory & Explanation & Statistic & Example\\
    \midrule 
  
     \multirow{3}*{\shortstack{Describe \\ Issue}} & Describe error scenario & Describe where and how an error occurs directly & 50(19.8\%) & \textit{``As-is it throws unchecked exceptions on unexpected charsets. This is a problem because it can cause a misbehaving webserver to crash the client.''} \\
    
    & Introduce issue report & Describe issues mainly by citing errors/defects or warnings from quality assurance tools & 11(4.4\%) & \textit{``remove warnings found by errorprone. [...] CallTest.java:2056: warning: [UnnecessaryParentheses] Unnecessary use of grouping parenthese [...]''} \\
    
     & Describe shortcoming & Highlight the shortcomings or weaknesses in the current implementation, which is the motivation to make this commit & 9(3.6\%) & \textit{``I'm unhappy with java.io: No timeouts [...] Features like mark/reset and available() are clumsy [...]''} \\
    \midrule
    
    \multirow{3}*{\shortstack{Illustrate \\ Requirement}} & Usage need & Describe specific needs or requirements of users in software development & 11(4.4\%) & \textit{``Error-prone only works on pre-12 at the moment and we need this configuration to apply for all JDKs''} \\
    
    & Out of date & Indicate the obsolescence of some features or code & 24(9.5\%) & \textit{``Remove outdated key. The `spring.metrics. export.redis.aggregate-key-pattern' is no longer defined but was still referenced in the documentation.''} \\
    
     & Runtime or development environment change &  Indicate an adaptation to the current code development or runtime environment & 11(4.4\%) & \textit{``API has changed, fixing the example''} \\
    \midrule
    
     \multirow{2}*{\shortstack{Describe \\ Objective}} & To solve the defects& Make explicit that the purpose of a change is to resolve a defect & 9(3.6\%) & \textit{``Fix concurrent problem of zookeeper configcenter, wait to start until cache being fully populated''}\\
    
     & For property promotion & Describe the improvement of an author’s code implementation, e.g, functional improvement or nonfunctional goals directly & 13(5.2\%) & \textit{``AndroidLog: Added [...] methods for easier subclassing.''} \\
    \midrule
    
     \multirow{4}*{\shortstack{Imply \\ Necessity}} & Conventions and standards & Describe or refer to any conventions or standards that are the basis for a change, thus proving the sound rationale of the change & 15(6.0\%) & \textit{``it is common to add tests to the same package as the class under test''} \\
    
     & Relation to prior commits & Explain the relationship between the current commit and any commits that were already merged into the repository & 9(3.6\%) & \textit{``the code was changed by commit <other url> but unfortunately the test was not part of the commit''}\\
    
     & Relation to an implemented feature &  Relate to an existing feature, and this relationship provides the context of the new commit & 9(3.6\%) &  \textit{``a short step on the road to HTTP body format agnostic support.''} \\
    
     & Improvements and benefits & Describe the need for a change by explaining the improvements and benefits that the change will bring  \textbf{indirectly} & 39(15.5\%) & \textit{``Use custom exception type [...]. Since we omit the stack trace, this more clearly indicates the source being from Retrofit's mock behavior''} \\
    \midrule
    
     \multirow{6}*{\shortstack{Missing \\ Why}} & Test cases &  Involve adding test cases to the repository & 4(1.6\%) & \textit{``tests for canceling async requests.''}\\
     & Typographic fixes & Involve the correction of typographic errors & 7(2.8\%) & \textit{``fix typo a->an''}\\
     & Text file changes &  Involve changes made only in text files & 13(5.2\%) & Changes in special function files, such as ``ChangeLog'', ``README''\\
     & Annotation changes & Refer to the motivation to modify the content of annotations & 5(2.0\%) & \textit{``add docs about null responses''}\\
     & Code refactoring & Involve refactoring and formatting of code & 15(6.0\%) &  \textit{``Polish pom.xml. Apply consistent formatting, drop JDK 8 support and cleanup repo [...]''}\\
     & Version management & Include changes that involve version management, such as the updating of version numbers  & 5(2.0\%) &  \textit{``prepare version 2.8.1''} \\
    \bottomrule 
    \end{tabular} 
\end{adjustbox}
\label{Why (sub)categories information}
\end{table*}
